# Supplementary material for: Numerical shape and topology optimization of regions supporting the boundary conditions of a physical problem
Source: arXiv:2502.19510 source file (2025-02-26)
Supplement: Supplementary file 1 [file Appendix.tex]

%\appendix
%%%%%%%%%%%%%%%%%%%%%%%%%
%\section{Some facts from tangential calculus}
%%%%%%%%%%%%%%%%%%%%%%%
%
%\begin{corollary} \label{theorem.Appendix.StandardChangeVariables}
%    Let $\Omega \subset \mathbb{R}^d$ be a bounded, Lipschitz domain, and let $\phi$ be a diffeomorphism from $\mathbb{R}^d$ onto itself. Then, a measurable function $f : \mathbb{R}^d \rightarrow \mathbb{R}$, belongs to $L^1(\phi(\partial \Omega))$ if and only if $f\circ \phi \in L^1(\partial \Omega)$, and:
%    \begin{equation}
%        \int_{\phi(\partial \Omega)} f ~ \d x = \int_{\Omega} |\det (\nabla \phi)| ~ f \circ \phi ~ \d x,
%    \end{equation}
%    where $\nabla \phi$ is the Jacobian matrix of $\phi$.
%\end{corollary}
%
%\begin{corollary} \label{theorem.Appendix.SurfaceChangeVariables}
%    Let $\Omega \subset \mathbb{R}^d$ be a bounded, Lipschitz domain, and let $\phi$ be a diffeomorphism from $\mathbb{R}^d$ onto itself. Then, a measurable function $f : \mathbb{R}^d \rightarrow \mathbb{R}$, belongs to $L^1(\phi(\partial \Omega))$ if and only if $f\circ \phi \in L^1(\partial \Omega)$, and:
%    \begin{equation}
%        \int_{\phi(\partial \Omega)} f ~ \d x = \int_{\partial \Omega} \det (\nabla \phi)|(\nabla \phi)^{-T} n| ~ f \circ \phi ~ \d x,
%    \end{equation}
%    where $\nabla \phi$ is the Jacobian matrix of $\phi$.
%\end{corollary}
%
%\begin{proposition} \label{prop.TangentialIntByParts}
%Let $\Omega \subset \mathbb{R}^d$ be a smooth bounded domain with boundary $\partial \Omega$. Let $u \in H^1(\partial \Omega)^d$ and $\theta \in H^1(\partial \Omega)^d$. Then:
%\begin{equation}
%    \int_{\partial \Omega} u \nabla_{\partial \Omega} \cdot \theta ~ \d s = \int_{\partial \Omega} (- \theta \cdot \nabla_{\partial \Omega} u + \kappa u \theta \cdot n) ~ \d s
%\end{equation}
%\end{proposition}
%
%\section{Green's identities}
%The following are simple consequences of the usual Green's identities.
%\begin{proposition} \label{prop.GreensIdentities}
%Let $\Omega$ be a domain with smooth boundary. They are valid for deformations $\theta \in \Winfty$, functions $w \in H^1(\Omega)$, and vector fields $a, b \in H^1(\Omega)^d$.
%\begin{equation}
%    \int_\Omega w \nabla \cdot \theta ~ \d x = \int_{\partial \Omega} w \theta \cdot n ~ \d s - \int_\Omega \theta \cdot \nabla w ~ \d x,
%\end{equation}
%and
%\begin{equation}
%    \int_{\Omega} \nabla \theta a \cdot b ~ \d x = \int_{\partial \Omega} (a \cdot n) (\theta \cdot b) ~ \d s - \int_\Omega (\dv a )(b\cdot \theta) ~ \d x - \int_\Omega (\nabla b) a \cdot \theta ~ \d x .
%\end{equation}
%\end{proposition}
%
